# Supplementary material for: Observation of three-photon bound states in a quantum nonlinear medium
Source: arXiv:1709.01478 source file (2017-11-10)
Supplement: Supplementary file 1 [file SI_full.pdf]

**Contents**

**S1. Materials and Methods** 1
A. Atom loading and preparation 1
B. Correlation and phase measurement setup 2
C. *Ab initio* calculation of the initial slope of the correlation functions 3

**S2. Supplementary Text** 3
A. Microscopic Model 3
B. Effective Field Theory 5
1. Estimating the Three-Body Force 5
2. Comparison Between EFT, Numerical Simulations, and Experimental Data 7
C. Formation of $N$-Body Bound States 8
D. Finite Rate Corrections to Theory 9
E. Dissipative Corrections to Theory 11

**Supplementary References** 12

# S1. MATERIALS AND METHODS

## A. Atom loading and preparation

The $^{87}$Rb atoms are loaded from a 3D magneto-optical trap (MOT) into a 1064 nm crossed dipole trap. The dipole trap is modulated with a period of 40 $\mu$s and 80 % duty cycle. A $\sim 6$ $\mu$s long probe pulse is sent to the atomic cloud while the dipole trap is off to avoid inhomogeneous AC Stark shift and the anti-trapping of the Rydberg atoms. The modulation of the trap and therefore the measurements last for 120 ms before a new atomic cloud is loaded. The average resonant optical depth along the atomic cloud is 36. The root-mean-square (RMS) length of the medium is $\sigma_{\rm ax} = 32$ $\mu$m. The atoms are optically pumped into the hyperfine ($F$) and magnetic ($m_F$) sublevel $|g\rangle = |5S_{1/2}, F = 2, m_F = 2\rangle$. The weak coherent probe light is coupled to the Rydberg state, via an intermediate state $|e\rangle = |5P_{3/2}, F = 3, m_F = 3\rangle$, of linewidth $\Gamma/2\pi = 6.1$ MHz, by means of a counter-propagating control field that is detuned by $\Delta$ below the resonance frequency of the upper transition, $|e\rangle \to |r\rangle = |100S_{1/2}, m_J = 1/2\rangle$, in the presence of a 3 G magnetic field along the long axis of the cloud. Probe and control counter-propagate along the quantization axis. The blockade radius $r_B$ defined as $\left(C_6 \frac{2|\Delta|}{\Omega_c^2}\right)^{\frac{1}{6}}$ is 20 $\mu$m, where $C_6/\hbar = 2\pi \times 56.4$ THz$\cdot$($\mu$m$^6$) is the van der Waals coefficient and $\Delta = 30$ MHz is the one-photon detuning.

### B. Correlation and phase measurement setup

In Fig. 1A of the main text, the first two beamsplitters are polarizing beamsplitters (PBS), and the last one is a 8:92 pellicle beamsplitter to minimize loss of the probe photons. There are polarization optics (not shown in the figure) before the first PBS to clean up the polarization of the probe, after which a half-wave plate is placed before each PBS to balance the detection rates on the three detectors.

We obtain the phase by performing a heterodyne measurement by mixing the transmitted probe light with a local oscillator (LO) at detector $D_3$ as shown in Fig. 1A. The LO is blue detuned by 79 MHz from the probe laser and this frequency difference is generated by an acousto-optic modulator (AOM). Afterwards, the two beams are sent through their own optical fibers. In order to take out the phase fluctuations caused by the fibers, we interfere the probe and LO, and trigger the single-photon detectors with the beatnote, which serves as a time zero for each probe pulse. Unlike the probe, the LO does not propagate through the atomic cloud, causing an additional phase drift on a time scale of tens of milliseconds. We keep track of the overall phase drift by fitting the unconditional phase for each time interval of $\sim 10$ ms. The interpolation of this time-dependent unconditional phase is added to each detection event on detector $D_3$ (phase measurement) to enable averaging over hours for the conditional phase measurements. Since we only detect one output port of the pellicle beamsplitter, the intensity noise cannot be canceled as in a balanced detection. Therefore, the LO counts is kept about four times of that of the probe on detector $D_3$.

To produce the unconditional phase measurement in Fig. 1C of the main text, we modulate probe-dipole trap for 5 ms. The sequence is adjusted such that during this 5 ms measurement time, the average optical depth is the same as a usual sequence. After that, we shut off the dipole trap and allow the atomic cloud to expand for 1 ms. We then measure the unconditional phase for 4 ms and use it as the phase reference.

The rate-dependent $\phi^{(1)}$ in Fig. 1D of the main text is generated by alternating relatively strong and weak (input photon rate of 0.5 $\mu s^{-1}$) pulses. The weak pulse serves as the phase reference, and a constant offset is applied to all the points such that the linear fit crosses the origin.

By conditioning on detecting two probe photons at time $t_1$ and $t_2$, and performing a phase measurement at time $t_3$, we directly measure $\tilde{\phi}^{(3)}(t_1, t_2, t_3) - \tilde{\phi}^{(2)}(t_1, t_2) - \tilde{\phi}^{(3)}_{ref}$. From the same data, by conditioning on detecting one probe photon, we obtain $\tilde{\phi}^{(2)}(t_1, t_2) - \tilde{\phi}^{(1)}(t_1) - \tilde{\phi}^{(2)}_{ref}$, where $\tilde{\phi}^{(N)}_{ref}$ denotes the phase reference of the directly measured phase conditioning on detecting N-1 probe photons. We can use the local unconditional phase when the phase measurement is performed as the reference, as in Fig. S1, namely, $\tilde{\phi}^{(3)}_{ref} = \tilde{\phi}^{(1)}(t_3)$ and $\tilde{\phi}^{(2)}_{ref} = \tilde{\phi}^{(1)}(t_2)$. For uncorrelated photons, N-photon phase can be written as the sum of the one-photon phase, e.g. $\tilde{\phi}^{(3)}(t_1, t_2, t_3) \xrightarrow{|t_i - t_j| \to \infty, \forall i \neq j} \tilde{\phi}^{(1)}(t_1) + \tilde{\phi}^{(1)}(t_2) + \tilde{\phi}^{(1)}(t_3)$. Therefore, at large $|\tau|$, both conditional phases in Fig. S1 are expected to go to 0. However, there is small disagreement

between the unconditional and the conditional phase with well separated photons. The conditional phases vary at a time scale of a few tens of microseconds, much slower than the bound state physics. Additionally, the mismatch is only less than 20 % of the phase of the concurrent photons. Therefore, we do not believe the phase offset at large $\tau$ to have significant impact on our main results.

In the main text, on the other hand, we use its own average value when the two photons are far away from each other as the phase reference $\tilde{\phi}^{(2)}_{ref}$. $\tilde{\phi}^{(3)}_{ref}$ includes both the phase of the uncorrelated photons and the phase conditioning on detecting one probe photon, namely, $\tilde{\phi}^{(3)}_{ref} = \tilde{\phi}^{(1)}(t_3) - (\tilde{\phi}^{(2)}(t_1,t_2) - \tilde{\phi}^{(1)}(t_1) - \tilde{\phi}^{(2)}_{ref})$. Assuming all detectors are interchangeable, this leads to $\tilde{\phi}^{(3)}(t_1,t_2,t_3) - (\tilde{\phi}^{(1)}(t_1) + \tilde{\phi}^{(1)}(t_2) + \tilde{\phi}^{(1)}(t_3))$, defined as $\phi^{(3)}(t_1,t_2,t_3)$ in the main text.

### C. *Ab initio* calculation of the initial slope of the correlation functions

We independently measure OD, the control Rabi frequency $\Omega_c$, the one-photon detuning $\Delta$, the root-mean-square length of the medium $\sigma_{\rm ax}$ and the group delay (the propagation time of the photon in the medium). The blockade radius $r_B$ is calculated from the measured $\Omega_c$, $\Delta$ and the known $C_6$ coefficient. The optical depth per blockade radius $\text{OD}_B$ is calculated from the measured OD and RMS length of the cloud $\sigma_{\rm ax}$ assuming a Gaussian atomic density profile. The population decay rate $\Gamma$ is taken from the known natural linewidth. The group velocity $v_g$ is calculated from the measured group delay and $\sigma_{\rm ax}$. We then use these quantities to calculate the scattering length and $\tau_{2,3}$.

## S2. SUPPLEMENTARY TEXT

### A. Microscopic Model

These experiments can be understood schematically in terms of the multi-particle transport problem illustrated in Fig. S2. A coherent state of light is incident on the quantum nonlinear optical medium formed from Rydberg atoms. Due to the interactions inside the medium, the output light exhibits multi-photon entanglement and correlations. Developing a full theoretical description of the transmitted light field is challenging even in the limit of a few-photons because the photons must be treated as a continuous quantum field. Nevertheless significant simplifications in the theory are possible due to the large separation of scales between the microscopic degrees of freedom and the emergent scales present in the correlations of the output light. We recently developed an effective field theory (EFT) description of this transmission problem by taking advantage of this large separation of scales [S1]. This EFT framework forms the basis of our theoretical analysis of the three-photon transmission problem studied in this work.

As the starting point for our theory we use a continuum description of the problem which first coarse grains over the atomic density to define local continuous quantum fields $\psi_g(z)$, $\psi_p(z)$, and

$\psi_s(z)$ for the photons, intermediate atomic excited state, and Rydberg state, respectively. These operators satisfy bosonic commutation relations $[\psi_a(z), \psi_b^\dagger(z')] = \delta_{ab}\delta(z-z')$. In describing the transmission of the photonic field $\psi_g$, we integrate out the other transverse propagating photonic degrees of freedom to arrive at a master equation description of the problem ($\hbar = 1$)

$$\dot{\rho} = -i\int dz[\mathcal{H}_0(z) + \mathcal{H}_{\rm int}(z), \rho] + \frac{\Gamma}{2}\int dz\mathcal{D}[\psi_p(z)]\rho + \frac{\gamma_s}{2}\int dz\mathcal{D}[\psi_s(z)]\rho, \tag{S1}$$

$$\mathcal{H}_0(z) = \begin{pmatrix} \psi_g(z) \\ \psi_p(z) \\ \psi_s(z) \end{pmatrix}^\dagger \begin{pmatrix} -ic\partial_z & g(z) & 0 \\ g(z) & -\Delta & \Omega_c/2 \\ 0 & \Omega_c/2 & -\delta \end{pmatrix} \begin{pmatrix} \psi_g(z) \\ \psi_p(z) \\ \psi_s(z) \end{pmatrix}, \tag{S2}$$

$$\mathcal{H}_{\rm int} = \int dz' \psi_s^\dagger(z)\psi_s^\dagger(z')V(z-z')\psi_s(z')\psi_s(z), \tag{S3}$$

where $\mathcal{D}[A]\rho = -\{A^\dagger A, \rho\} + 2A\rho A^\dagger$ is a trace-perserving superoperator, $\mathcal{H}_0$ is the non-interacting Hamiltonian density written in the rotating frame, and $\mathcal{H}_{\rm int}$ is the Rydberg interaction Hamiltonian density. The non-interacting theory is parameterized in terms of the control field Rabi frequency $\Omega_c$, the fullwidth of the intermediate state $\Gamma$, the fullwidth of the Rydberg state $\gamma_s$, the detuning $\Delta = \omega_{ps} - \omega_c$ between the control field frequency $\omega_c$ and the Rydberg-intermediate state transition frequency $\omega_{ps}$, and the two-photon detuning $\delta = \omega_p + \omega_c - \omega_{gs}$ between the sum of $\omega_c$ and the input probe frequency $\omega_p$ and the ground to Rydberg state transition frequency $\omega_{gs}$. The single-photon Rabi frequency for the probe $g(z)$ is proportional to the square root of the atomic density $n(z)$, with the proportionality constant determined by the resonant optical depth $\text{OD} = \int dz\, 4\,[g(z)]^2/\Gamma c$. We parameterize the density by a Gaussian profile $n(z) \propto \exp(-z^2/2\sigma_{\rm ax}^2)$, where $\sigma_{\rm ax}$ is the RMS axial width of the cloud. Finally, we approximate the Rydberg interactions by their long-range van der Waals tail $V(r) = C_6/r^6$.

An important simplification of this problem is provided for photonic input states with a low photon rate, where the evolution can be described solely in terms of the dynamics induced by the effective non-Hermitian Hamiltonian [S2]

$$\mathcal{H}_{\rm eff} = \mathcal{H}_0 + \mathcal{H}_{\rm int} - i\frac{\Gamma}{2}\psi_p^\dagger\psi_p - i\frac{\gamma_s}{2}\psi_s^\dagger\psi_s. \tag{S4}$$

The decay terms can be incorporated into $\mathcal{H}_0$ through the replacements $\Delta \to \Delta + i\Gamma/2$ and $\delta \to \delta + i\gamma_s/2$. This approximation relies on the fact that the corrections to the non-Hermitian Hamiltonian evolution from the recycling terms in the master equation, i.e., the so-called "quantum jumps," are suppressed by higher powers of the polariton density in the medium (see Ref. [S3] for a similar argument applied to a cavity model). Since the experiments are operated in the limit of low polariton densities in the medium, we are justified in neglecting these quantum jump processes. We present a more detailed discussion of these effects in Sec. S2 E.

## B. Effective Field Theory

For sufficiently low-energy scattering of two-particles, the dynamics of the Rydberg polaritons are described by the renormalized Lagrangian density [S4]

$$\mathcal{L}_0 = \psi^\dagger \Big[ i\partial_t + iv_g\partial_z - \frac{1}{2m_0}\partial_z^2 \Big]\psi_\mu + \frac{1}{m_0 a}\psi^\dagger\psi^\dagger\psi\psi, \tag{S5}$$

$$v_g = \frac{d\epsilon_D(k)}{dk}\Big|_{k=k_0}, \quad \frac{1}{m_0} = \frac{d^2\epsilon_D(k)}{dk^2}\Big|_{k=k_0}, \tag{S6}$$

where $a$ is the one dimensional scattering length, $\epsilon_D(k)$ is the dispersion relation of the dark-state polaritons obtained from the non-interacting part of $\mathcal{H}_{\mathrm{eff}}$, $v_g$ is the EIT group velocity, and $m_0$ is the effective mass.

This EFT is exactly solvable in 1D and, for attractive interactions ($a > 0$), it has one $N$-body bound state for every $N$ [S5, S6]. The properties of the three-body bound state are discussed in the main text. At low-momenta, the lowest order correction to this theory is given by a three-body interaction [S7]

$$\mathcal{L} = \mathcal{L}_0 - V_3, \tag{S7}$$

$$V_3 = \frac{h_3}{36}\psi^{\dagger 3}\psi^3. \tag{S8}$$

This term, although irrelevant for low-energy, few-body observables in the scaling limit ($|a| \to \infty$) [S8], has important physical consequences at any finite momentum scale. As discussed in the main text, we can understand the origin of three-body interactions in the Rydberg-EIT system at a qualitative level as arising from the physics of Rydberg blockade. When more than two photons are within a blockade radius from each other, their interaction energy is suppressed due to the blockade effect. This leads to an effective three-body force with the opposite sign from the two-body force as was shown in our recent work [S1] and Ref. [S9]. Although analytic expressions for the three-body interaction were derived in these works, these derivations neglected non-perturbative effects in the renormalization of the microscopic model. In the section below, we provide an alternative estimate of the three-body force that fully accounts for these corrections, but in a simplified version of the microscopic model.

### 1. *Estimating the Three-Body Force*

In this section, we outline a procedure to estimate the value of the three-body force in the EFT by matching its prediction for the dimer-polariton scattering length to a simplified version of the microscopic model. Here the dimer is the shallow two-body bound state with the binding energy

$$E_D = -\frac{1}{m_0 a^2}. \tag{S9}$$

Before proceeding to the three-body problem, we first note that the microscopic two-body problem can be solved via an effective Schrödinger equation for a particle with mass $m_0$ and two-body

interactions of the form [S10, S4]

$$U(\omega, r) = \frac{U(\omega, 0)}{1 + r^6/r_b^6(\omega)}, \tag{S10}$$

$$U(\omega, 0) \approx \frac{\Omega_c^2}{2\Delta} - \omega, \tag{S11}$$

where $r$ is the relative position of the two photons, $\omega$ is the total frequency of the incoming photons and the approximate inequality for $U(\omega, 0)$ applies in the experimentally relevant regime of $\Delta \gg (\Omega_c, \Gamma) \gg \gamma_s$. Here we have defined the frequency dependent, complex valued blockade radius $r_b(\omega) = [C_6/U(\omega, 0)]^{1/6}$, which is related to the blockade radius $r_B$ used in the main text and defined in Sec. S1 A through the identity $r_B \approx |r_b(0)|$.

To solve the three-body problem we introduce a simplified description of the full microscopic problem that is easier to treat analytically and numerically. In particular, we replace the effective interaction potential $U(\omega, r)\delta(r - r')$ in the integral equations for the two and three-body scattering amplitudes by a non-local, so-called "separable" potential

$$U(\omega, r, r') = u_0(\omega)u(r)u(r'), \tag{S12}$$

$$u_0(\omega) = \int dr U(\omega, r) = \frac{2\pi}{3} U(\omega, 0) r_b(\omega). \tag{S13}$$

Here $r$ ($r'$) are the relative positions of the two incoming (outgoing) particles in the scattering process. Note that $U(\omega, r, r')$ is not to be confused with $U(r, r')$ defined in Fig. 4(a) of the main text. In our calculations, we take a square well potential in momentum space, i.e., $u(r) = \Lambda \operatorname{sinc}(\pi\Lambda r)$ with $\Lambda \sim 1/r_B$ chosen to match the microscopic two-body scattering length $a$. The separable approximation allows the two-body $T$-matrix to be analytically solved and leads to several key simplifications in the implementation of numerical solutions of the Faddeev equations for the three-body scattering amplitudes of Rydberg polaritons [S12].

To fix the value of $h_3$ we match the dimer-polariton scattering length (obtained numerically) in the EFT to that of the simplified microscopic model. To regularize UV divergences in our solution of the EFT in Eq. (S7), we also take a separable form for the effective two and three-body interactions

$$V_2(r, r') = \frac{2}{m_0 a} v(r)v(r'), \tag{S14}$$

$$V_3(\boldsymbol{r}, \boldsymbol{r}') = h_3 v(r_1)v(r_2)v(r_1')v(r_2'), \tag{S15}$$

where $r$ ($r'$) are the relative coordinate of the two incoming (outgoing) polaritons. For the three-body case, we use the convention that for an incoming polariton with coordinate $z_1$ and an incoming dimer with coordinates $(z_2, z_3)$, $r_1 = z_1 - z_2$ and $r_2 = z_1 - z_3$ and similarly for the outgoing coordinates. In the EFT we take a square well potential in real space $v(r) = \theta(\delta r - |r|)/2\delta r$ with $\theta(\cdot)$ the Heaviside step function. The potential is chosen as a square well because this is the form we use for the interactions when solving the transmission problem using the EFT. Defining the interaction parameter $\varphi = \mathrm{OD}_B\Gamma/4\Delta = g^2 r_B/c\Delta$, we parameterize the range of the effective potentials as $\delta r = \alpha r_B/\varphi$ for $\alpha \lesssim 1$. Since the scattering length in the

experimentally relevant regime of small $\varphi$ satisfies $a \approx r_B/\varphi^2$ [S4], we have $\delta r/a \approx \alpha\varphi \ll 1$, such that these potentials can be well approximated by contact interactions at low-momentum. To perform the matching, we fix $h_3 m_0 = \beta\varphi^2$ for some choice of $\beta$ and then adjust the range of the potential via $\alpha$ to match the scattering amplitudes. For Fig. 4 in the main text we chose $\beta = 13.5$ near the value obtained from our previous analytic predictions for the three-body force [S1, S9]. Performing the matching calculation we found $\alpha \approx 0.1$ for the experimentally relevant range of $\varphi$. Although the precise choice of matching procedure is somewhat arbitrary, what is important is that the physical observables are independent of these details. We have verified that the predicted values of the ratio $\phi_3(0,0)/\phi_2(0)$ from the EFT vary by less than 5 % when the choice of $\beta$, with $\alpha$ obtained from matching, is varied within 50 %.

### 2. *Comparison Between EFT, Numerical Simulations, and Experimental Data*

To solve the transmission problem we use a modified version of the EFT that takes into account the spatial inhomogeneity of the atomic density. Most notably, we use a local density approximation (i.e., each parameter is defined in terms of the local value of $g(z)$) and transform into a moving frame through the coordinate transformation [S1]

$$\bar{z} = t - \int_0^z dz' \frac{1}{v_g(z')}, \tag{S16}$$

$$\tau = z, \tag{S17}$$

which transforms the Lagrangian to the form

$$\mathcal{L} = \psi^\dagger \left[ i v_g(\tau)\partial_\tau - \frac{\partial_{\bar{z}}^2}{2m_0(\tau)v_g^2(\tau)} \right]\psi + \frac{\psi^{\dagger 2}\psi^2}{m_0(\tau)a(\tau)v_g(\tau)} - \frac{h_3(\tau)}{36\, v_g^2(\tau)}\psi^{\dagger 3}\psi^3, \tag{S18}$$

where we have rescaled the field $\psi(z) \to \psi(\bar{z})/\sqrt{v_g(\tau)}$ such that $[\psi(\bar{z}), \psi^\dagger(\bar{z})] = \delta(\bar{z} - \bar{z}')$ and we have neglected higher-order derivatives involving $\partial_\tau$ as their effect is suppressed due to the presence of the linear time derivative. This EFT is a more convenient formulation of the transmission problem because the parameters now depend on "time" $\tau$, which only appears with a single derivative. As a result, this theory can be solved by treating it as a time-dependent Hamiltonian problem. Furthermore, it illustrates that the transmission through the medium can be mapped to a quantum quench, where the duration of the time evolution following the quench is given by the EIT group delay $\tau_d = \int dz \frac{1}{v_g(z)}$ [S1, S10, S14]. When numerically solving for the transmission using Eq. (S18), we regularize the two and three-body contact interactions by taking symmetrized, local and non-separable square well interaction potentials

$$V_2(\bar{z}_i, \bar{z}_j) = \frac{2}{m_0 a} v(\bar{z}_i - \bar{z}_j), \tag{S19}$$

$$V_3(\bar{z}_1, \bar{z}_2, \bar{z}_3) = \frac{h_3}{3}\left[ v(\bar{z}_1 - \bar{z}_2)v(\bar{z}_1 - \bar{z}_3) + v(\bar{z}_1 - \bar{z}_2)v(\bar{z}_2 - \bar{z}_3) + v(\bar{z}_1 - \bar{z}_3)v(\bar{z}_2 - \bar{z}_3) \right], \tag{S20}$$

where $v(r) = \theta(\delta r - |r|)/2\delta r$, $h_3 = \beta\varphi^2/m_0$, $\delta r = \alpha r_B/\varphi$ and $\alpha$ and $\beta$ were determined via the matching procedure for separable potentials described in the previous section. In contrast

to the separable potentials defined in Eq. (S14)-(S15), here we have suppressed the dependence on the outgoing coordinates as, due to the locality assumption, the outgoing coordinates are constrained to be equal to the incoming coordinates.

In Fig. S3(a-b) we compare the predictions from numerical solutions of Eq. (S18) for the transmission through a finite medium to full numerical simulations that account for the microscopic form of the Rydberg interactions [S15]. We see good agreement between the numerics and the EFT at intermediate times. The deviations at short times are due to the breakdown of the low-energy assumption and the deviations at long times arise from the finite length of the medium [S1]. We use the initial condition outside the medium of a uniform state with unit amplitude. We find that including the three-body interaction improves the agreement with $\phi_3(t,0)$ at intermediate times. Similar to Fig. 3 in the main text, we see that including the three-photon force reduces the ratio $\phi_3(0,0)/\phi_2(0)$, where $\phi_2(t)$ is the two-photon phase. Table S1 shows the ratio $\phi_3(0,0)/\phi_2(0)$ for the three different models, where we see that including the three-body force is able to account for the deviation of this ratio below 3. Despite the disagreement between the values of $\phi_3(t,0)$ in the simulations and the EFT at short times seen in Fig. S3, we find that the ratio $\phi_3(t,0)/\phi_2(t)$ is roughly independent of $t$ near the origin, which justifies the comparison.

In Table S2 we compare the theoretical predictions from the EFT and the simulations against the measured values of $\phi_3(0,0)/\phi_2(0)$ from Fig. 4 in the main text. Here $\langle\varphi\rangle = \tau_d^{-1}\int dz \varphi(z)/v_g(z)$ is the average value of $\varphi(z) = \mathrm{OD}_B\Gamma/4\Delta = g^2(z)r_B/c\Delta$ weighted by the time spent in each region. As mentioned in the main text, we fit the two-photon detuning $\delta$ within the experimental uncertainty $\delta/2\pi = 0.0 \pm 0.5$ MHz by matching the measured value of $\phi_2(0)$ to the simulations. All other parameters are determined from independent measurements without fitting. Although $\phi_2(0)$ and $\phi_3(0,0)$ are sensitive to the precise value of $\delta$, we find that the theoretical prediction for the ratio $\phi_3(0,0)/\phi_2(0)$ varies by less than 5 % when varying $\delta$ within the experimental uncertainty. We see that the EFT with the three-body force gives good agreement with both the data and the simulations, while we can clearly rule out the EFT without the three-body force.

### C. Formation of $N$-Body Bound States

In this section we present a general argument that the propagation through the medium leads to the formation of an $N$-body bound state near zero time delay between the polaritons. We first consider the two-body problem in a uniform medium. Defining the center of mass $R = (z_1+z_2)/2$ and relative $r = z_1 - z_2$ coordinates for the two polaritons, we expand the wavefunction in the eigenbasis of the EFT given in Eq. (S5) [S10]

$$\psi(t,R,r) = c_b e^{-|r|/a - iE_D t} + \int_0^\infty \frac{dq}{2\pi} c_q \psi_q(r) e^{-iq^2 t/m_0}, \tag{S21}$$

where the first term is the dimer wavefunction, $\psi_q(r) = (e^{iq|r|} + b_q e^{-iq|r|})/\sqrt{2}$ is the wavefunction for the two-body scattering states, $b_q = (iaq+1)/(iaq-1)$, and we work in the center of mass

frame so that $\partial_R \psi = 0$. The coefficients $c_b$ and $c_q$ are determined by initial conditions.

For a long medium, we can find the transmission analytically for $|r|/a \ll \sqrt{|E_D t|}$ using a saddle point expansion

$$\psi(t, R, r) \approx c_b e^{-|r|/a - iE_D t} + O(|E_D t|^{-1/2}), \tag{S22}$$

where the second term is due to the contribution from scattering states. The condition to neglect the second term for the transmitted light is

$$\tau_d |E_D| \approx 2\varphi^2 \mathrm{OD}\, \Gamma/\Delta \gg 1, \tag{S23}$$

where $\tau_d$ is the EIT group delay defined in Sec. S2 B 2. From this analysis we see that the dispersive nature of the scattering states results in the bound state dominating the transmission near the origin in the off-resonant, high OD limit.

To see how this argument generalizes to $N > 2$, we move to a relative coordinate system $r_1, \ldots, r_{N-1}$ (defined as any set of coordinates orthogonal to the center of mass coordinate $R = \sum_i z_i/N$). The general form for the evolution in the center of mass frame is given by

$$\psi(t, R, \boldsymbol{r}) = c_b \psi_b(\boldsymbol{r}) e^{-iE_N t} + \int \frac{dq}{2\pi} c_{bq} \psi_{bq}(\boldsymbol{r}) e^{-iE_{N-1}t - iq^2 t/2m_0} + \ldots, \tag{S24}$$

where $\psi_b$ is the wavefunction for the $N$-body bound state, $\psi_{bq}(\boldsymbol{r})$ is the wavefunction for a combined $(N-1)$-body bound state and a scattering state with relative momentum $q$, etc. Similar to the two-body problem, we can see that all contributions to $\psi$ besides $\psi_b$ will dephase with each other. As a result, the transmission is dominated by the bound state near the origin.

For the experiments studied in this work, $|E_N| \gtrsim \tau_d^{-1}$, therefore, it is important to also take into account the contributions from the scattering states in solving the transmission problem. To include these contributions when modeling the experiments, we perform numerical simulations of the two and three-photon wavefunction propagation equations derived from the EFT in Eq. (S18) including the inhomogeneous density profile.

### D. Finite Rate Corrections to Theory

The correlation functions analyzed above were taken with respect to the vacuum. In the experiment, the input state is a coherent state, which implies that $N$-particle correlation functions contain contributions from higher and lower particle-number manifolds. In the limit of a long coherent state pulse with a finite photon rate $R$, we now evaluate these corrections perturbatively in the normalized polariton density $R\tau_{\mathrm{int}}$. Here $\tau_{\mathrm{int}} \sim \tau_d$ is defined as the relative time difference over which the correlation functions do not factorize. We show that these finite rate corrections are small, which justifies our approximation of neglecting these corrections when comparing our theory to experimental data.

We write the input state as

$$e^{\alpha^2/2} |\mathcal{E}\rangle = |0\rangle + \alpha|1\rangle + \frac{\alpha^2}{\sqrt{2!}}|2\rangle + \frac{\alpha^3}{\sqrt{3!}}|3\rangle + \ldots, \tag{S25}$$

where

$$|n\rangle \;=\; \frac{(a^\dagger)^n}{\sqrt{n!}}|0\rangle,\;\; a^\dagger = \frac{1}{\sqrt{T}}\int dz\mathcal{E}(z)\psi_g^\dagger(z). \tag{S26}$$

Here $\mathcal{E}(z)$ is our input mode which we take to be a long uniform pulse of unit amplitude and duration $T$ from $z=0$ to $z=T$ (c=1). We write the output as

$$\begin{aligned} e^{\alpha^2/2}|\mathcal{E}\rangle \;=\; & |0\rangle + \sqrt{R}\int dz\mathcal{E}_1(z)\psi_g^\dagger(z)|0\rangle + \frac{R}{2}\int dz_1dz_2\mathcal{E}_2(z_1,z_2)\psi_g^\dagger(z_1)\psi_g^\dagger(z_2)|0\rangle \\ & + \frac{R^{3/2}}{6}\int dz_1dz_2dz_3\mathcal{E}_3(z_1,z_2,z_3)\psi_g^\dagger(z_1)\psi_g^\dagger(z_2)\psi_g^\dagger(z_3)|0\rangle + \ldots, \end{aligned} \tag{S27}$$

where the input photon rate is $R=\alpha^2/T$ and we define $g_n$ and $\phi_n$ via

$$\mathcal{E}_n(z_1,\ldots,z_n) \;=\; \sqrt{g_n(z_1,\ldots,z_n)}e^{i\theta_n(z_1,\ldots,z_n)}. \tag{S28}$$

Notice that $g_n$ and $\theta_n$ are different from the measured $g^{(n)}$ and $\phi_n$ because of the rate-dependent corrections. Neglecting dissipation leads to the normalization condition

$$e^{\alpha^2} = e^{\alpha^2}\langle\mathcal{E}|\mathcal{E}\rangle = 1 + R\int dz_1g_1(z_1) + \frac{R^2}{2}\int dz_1z_2g_2(z_1,z_2) + \ldots, \tag{S29}$$

which requires the identity

$$\int d^nz[g_n(z_1,\ldots,z_n)-1] = 0. \tag{S30}$$

One can show that including the decay rates in the effective Hamiltonian gives the leading order contribution to this integral on the order of $(\Gamma/\Delta)\tau_{\text{int}}^n$.

These identities allow us to prove that $g_n$ converges to $g^{(n)}$ in the limit of vanishing input rate $R\tau_{\text{int}}\to 0$. For example, for $g_2$ we find

$$\begin{aligned} g^{(2)}(z_1,z_2) &= \frac{1}{R^2}\langle\mathcal{E}|\psi_g^\dagger(z_1)\psi_g^\dagger(z_2)\psi_g(z_2)\psi_g(z_1)|\mathcal{E}\rangle \\ &= e^{-\alpha^2}[g_2(z_1,z_2)(1+\alpha^2+\ldots) + R\int dz[g_3(z_1,z_2,z) - g_2(z_1,z_2)] + \ldots], \end{aligned} \tag{S31}$$

Collecting all terms that are zeroth order in $R\tau_{\text{int}}$, we recover $g_2(z_1,z_2)$. In the limit $\Delta\gg\gamma$, this analysis also gives access to the first order correction in $R\tau_{\text{int}}$, which takes the general form

$$\begin{aligned} g^{(n)}(\tau_1,\ldots,\tau_{n-1}) &= g_n(\tau_1,\ldots,\tau_{n-1}) \\ &\quad + R\int d\tau(g_{n+1}(\tau_1,\ldots,\tau_{n-1},\tau) - g_n(\tau_1,\ldots,\tau_{n-1})). \end{aligned} \tag{S32}$$

For the single-photon phase, we can follow similar arguments to find

$$\frac{1}{\sqrt{R}}\langle\mathcal{E}|\psi_g(z)|\mathcal{E}\rangle = e^{i\theta_1} + R\int d\tau(\sqrt{g_2(\tau)}e^{i(\theta_2(\tau)-\theta_1)} - e^{i\theta_1}) + O(R^2\tau_{\text{int}}^2), \tag{S33}$$

and, generalizing to $\phi_n$,

$$\begin{aligned} &\frac{1}{R^{n-1/2}}\langle\mathcal{E}|\psi_g^\dagger(z_1)\cdots\psi_g^\dagger(z_{n-1})\psi_g(z)\psi_g(z_{n-1})\cdots\psi_g(z_1)|\mathcal{E}\rangle \\ &\quad = \mathcal{E}_{n-1}^*(z_1,\ldots,z_{n-1})\mathcal{E}_n(z_1,\ldots,z_{n-1},z) \\ &\quad + R\int dz'[\mathcal{E}_n^*(z',z_1,\ldots,z_{n-1})\mathcal{E}_{n+1}(z',z_1,\ldots,z_{n-1},z) \\ &\quad - \mathcal{E}_{n-1}^*(z_1,\ldots,z_{n-1})\mathcal{E}_n(z_1,\ldots,z_{n-1},z)]. \end{aligned} \tag{S34}$$

Using these formulas, we have explicitly evaluated the rate dependent corrections to $\phi_2$ and $\phi_3$ by numerically solving the four-photon transmission problem within the EFT. The results are shown in Fig. S4. For this data set ($\Delta/2\pi = 30$ MHz), the experiments were performed at a rate near 1 photon/$\mu s$. In this regime, the rate dependent corrections to the phase ratio are on the order of a few percent. This mostly rules out the rate dependent corrections as an explanation for the deviation of the phase ratio from three observed in the experiment. We find similar results for the other data sets. In Fig. 4B of the main text we compare the zero-rate predictions of the EFT to the experimentally measured values of $\phi_3(0,0)/\phi_2(0)$. In Fig. 4B of the main text we compare the zero-rate predictions of the EFT to the experimentally measured values of $\phi_3(0,0)/\phi_2(0)$.

### E. Dissipative Corrections to Theory

At large single-photon detunings $\Delta$ the dominant decay is due to the finite decoherence rate $\gamma_s/2$ of the Rydberg state. Experimentally we observe that the single-photon transmission through the medium is between 50 % and 90 %. Although we include the decay terms in the non-Hermitian Hamiltonian evolution, this large background decay inside the medium raises the question of whether we are justified in neglecting the recycling terms in the master equation. As was argued in Sec. S2 A, this approximation is indeed justified at sufficiently low polariton densities. More precisely, we find the requirement to neglect the recycling terms is given by $\gamma_s \tau_d R \tau_{\text{int}} \ll 1$. This condition is well satisfied for the experiment even when $\gamma_s \tau_d \sim 1$, which justifies our theoretical approach in which we neglect these corrections when comparing to experimental data.

We do not give a detailed proof of this result here, but note that this scaling can be understood intuitively because $\gamma_s \tau_d$ is the expected number of decay events, or "quantum jumps," per photon during the transmission through the medium, while $R\tau_{\text{int}}$ is the probability of having a second photon within the interaction range of the first when the quantum jump occurs, i.e., the normalized polariton density. Thus, under the condition $\gamma_s \tau_d R \tau_{\text{int}} \ll 1$, the quantum jumps typically happen when there are no other polaritons nearby with which to interact. In this case, the interacting correlation functions will have a small contribution from quantum jump events from higher excitation number manifolds.

The role of quantum jumps associated with other loss processes inside the medium requires a separate treatment from the Rydberg decay because these effects appear in the polariton dynamics as momentum or frequency dependent loss (e.g., an imaginary mass term). In this case, the argument above does not apply because, for a long uniform pulse that has reached steady state inside the medium, these loss processes are always correlated with interactions between the polaritons. As a result, these quantum jump events do not average out when evaluating interacting correlation functions. It is not difficult to show, however, that these corrections are suppressed as the product of two small parameters $R\tau_{\text{int}}$ and $\Gamma/\Delta$, which justifies our neglect

of these quantum jump processes.

---


[S1] M. J. Gullans, J. D. Thompson, Y. Wang, Q.-Y. Liang, V. Vuletić, M. D. Lukin, and A. V. Gorshkov, Phys. Rev. Lett. **117**, 113601 (2016).

[S2] T. Peyronel, O. Firstenberg, Q.-Y. Liang, S. Hofferberth, A. V. Gorshkov, T. Pohl, M. D. Lukin, and V. Vuletic, Nature **488**, 57 (2012).

[S3] H. Carmichael, R. Brecha, and P. Rice, Opt. Commun. **82**, 73 (1991).

[S4] P. Bienias, S. Choi, O. Firstenberg, M. F. Maghrebi, M. Gullans, M. D. Lukin, A. V. Gorshkov, and H. P. Büchler, Phys. Rev. A **90**, 053804 (2014).

[S5] E. H. Lieb and W. Liniger, Phys. Rev. **130**, 1605 (1963).

[S6] J. B. McGuire, J. Math. Phys. **5**, 622 (1964).

[S7] E. Braaten and H. W. Hammer, Phys. Rep. **428**, 259 (2006).

[S8] S. K. Adhikari, T. Frederico, and I. D. Goldman, Phys. Rev. Lett. **74**, 487 (1995).

[S9] K. Jachymski, P. Bienias, and H. P. Büchler, Phys. Rev. Lett. **117**, 053601 (2016).

[S10] O. Firstenberg, T. Peyronel, Q.-Y. Liang, A. V. Gorshkov, M. D. Lukin, and V. Vuletić, Nature **502**, 71 (2013).

[S11] A. V. Gorshkov, J. Otterbach, M. Fleischhauer, T. Pohl, and M. D. Lukin, Phys. Rev. Lett. **107**, 133602 (2011).

[S12] M. J. Gullans *et al.* in preparation.

[S13] P. F. Bedaque, H.-W. Hammer, and U. van Kolck, Phys. Rev. Lett. **82**, 463 (1999).

[S14] P.-É. Larré and I. Carusotto, Phys. Rev. A **92**, 043802 (2015).

[S15] M. J. Gullans, PhD Thesis, Harvard University, Cambridge, MA (2013).

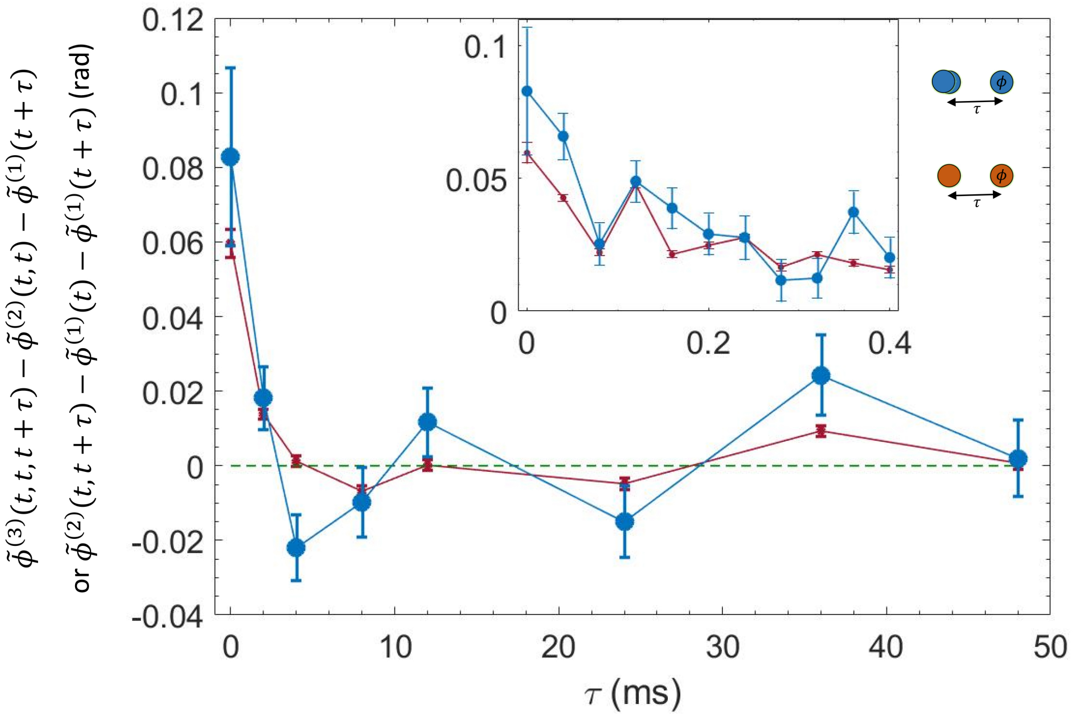


FIG. S1: **The long range behavior of the conditional phase referenced to the local unconditional phase.** The blue and brown data represent $\tilde{\phi}^{(3)}(t,t,t+\tau)-\tilde{\phi}^{(2)}(t,t)-\tilde{\phi}^{(1)}(t+\tau)$ and $\tilde{\phi}^{(2)}(t,t+\tau)-\tilde{\phi}^{(1)}(t)-\tilde{\phi}^{(1)}(t+\tau)$, respectively. The inset shows the same quantities at a shorter time scale. These data with $\tau$ much longer the probe pulse ($\sim 6\mu$s) are generated by taking detection events from different pulses. Data is the same as in Fig. 3 of the main text.

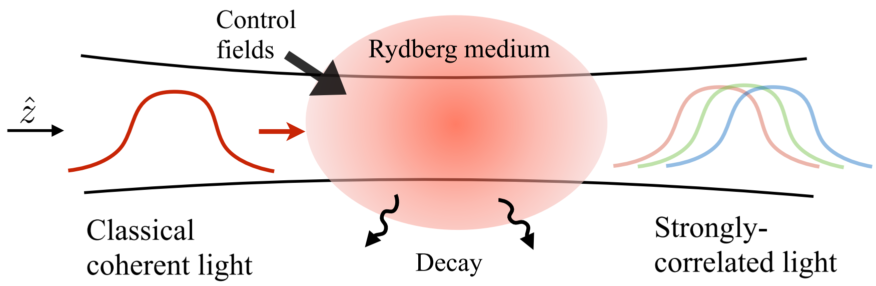


FIG. S2: **The scheme of the experiment.** This experiment can be conceptualized as a multi-particle transport problem whereby a classical coherent pulse of light enters the medium and becomes strongly-correlated on the output due to strong coherent and dissipative interactions inside the medium.

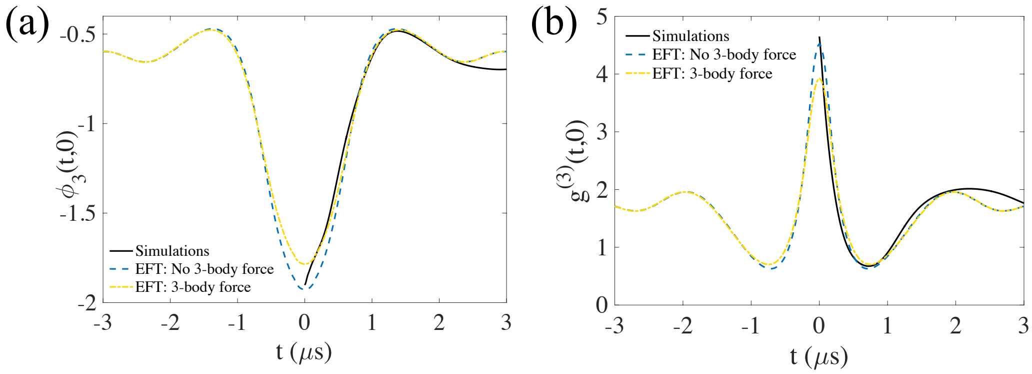


FIG. S3: **Comparison between EFT and simulations**. We compare the EFT predictions for the two and three photon transmission through a finite medium (see Ref. [S1]) and numerical simulations for (a) the three-photon phase $\phi_3(t,0)$ and (b) the three-photon amplitude $g^{(3)}(t,0)$. Here we took parameters similar to the current experiments, but with a uniform density profile of length 144 $\mu m$, a resonant OD=68, $\Omega_c/2\pi = 5$ MHz, $\Delta = 30$ MHz, $\gamma_s = 0$, and $r_B = 10$ $\mu$m.

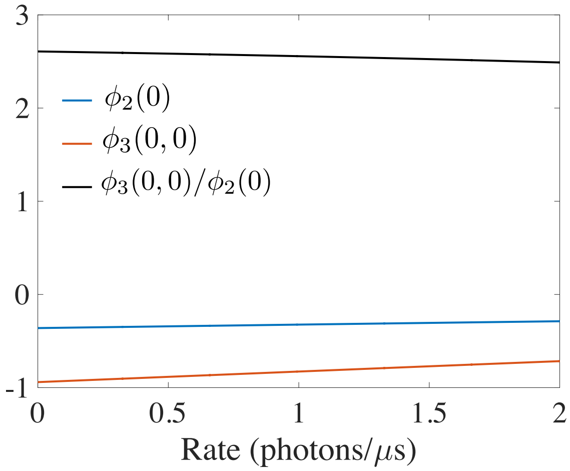


FIG. S4: **Rate dependent corrections within the EFT.** We use parameters from the 30 MHz data set. The experiment for this data set was performed at a rate of 1 photon/$\mu$s.

| Model | $\phi_3(0,0)/\phi_2(0)$ |
|---|---|
| Simulations | 2.90 |
| EFT: No 3-body force | 3.13 |
| EFT: 3-body force | $2.85 \pm .11$ |

TABLE S17: **Comparison of phase ratio between EFT and simulations.** Comparison for the prediction of the phase ratio near zero time delay between different models for parameters as in Fig. S3. The uncertainty in the EFT with the three-body force arises from the variations with the choice of matching conditions for the dimer-polariton scattering length.

| $\langle\varphi\rangle$=$\langle\mathrm{OD}_B\rangle\Gamma/4\Delta$ | 0.16 | 0.21 | 0.28 | 0.36 | 0.47 |
|---|---|---|---|---|---|
| Measured $\phi_3(0,0)/\phi_2(0)$ | $2.17 \pm .18$ | $2.45 \pm .15$ | $2.55 \pm .13$ | $2.33 \pm .27$ | $2.31 \pm .21$ |
| EFT: 3-body force | $2.64 \pm .18$ | $2.42 \pm .17$ | $2.48 \pm .11$ | $2.60 \pm .11$ | $2.52 \pm .13$ |
| Simulations | 2.77 | 2.66 | 2.72 | 2.63 | 2.60 |
| EFT: No 3-body force | 3.06 | 3.05 | 3.07 | 3.08 | 3.06 |
| Fitted $\delta$ ($2\pi$·MHz) | 0.6 | 0.6 | 0 | -0.2 | -0.4 |

TABLE S18: **Comparison of phase ratio between EFT, simulations and experimental data.** Comparison of measured $\phi_3(0,0)/\phi_2(0)$ presented in Fig. 4B of the main text to predictions from EFT with and without the three-body force and the simulations [S15]. We took an inhomogeneous Gaussian density profile with $\sigma_{\mathrm{ax}} = 32$ $\mu$m, $\gamma_s/2\pi = 200$ kHz, $\delta$ as shown (obtained from fitting the measured value of $\phi_2(0)$ to the simulations), and other parameters as given in the main text. The uncertainty in the EFT with the three-body force arises from the variations with the choice of matching conditions for the dimer-polariton scattering length.
